# Supplementary material for: Visualizing Ensemble Predictions of Music Mood
Source: arXiv:2112.07627 source file (2022-09-04)
Supplement: Supplementary file 1 [file appendix.tex]

method from previous paper:

E1. Horizontal first, add weighted average:

For example, green RF: top three, RF24, RF27, RF30.

     A := B := C := D;
     For model := { RF24, RF27, RF30 } do begin
         case model(input) do begin
        %  decision A: A := A + add model_accuracy; break;
        %  decision B: B := B + add model_accuracy; break;
        %  decision C: C := C + add model_accuracy; break;
        %  decision D: D := D + add model_accuracy; break;
         end
     end
     Choose the highest among A, B, C, D.

     Calculate the accuracy of ensemble RF-ensemble.

     For vertical ensemble, check all 14 models (7 best and 7 ensemble)
     Select N (out of 14) models, and use weighted ensemble again.

E2. Do the vertical first, then horizontal.

    Plot an ensemble curve and an best model curve.
    Choose N (out of 60) models, and use weighted ensemble again.

E3. Try the other ML-based methods.

E4. DONE: No need to do this again: decision tree based methods.

E5. Use the top two-layer models (3 models), use the weighted ensemble
of these three models.

E6. Use the top three-layer models (7 models), use the weighted ensemble
of these three models.

ML method 1-7: DT, bagging, adaboost, GBDT, XGB, RF, gcForest
raw results from the models:
30 sec	29 sec	28 sec	27 sec	26 sec	25 sec	24 sec	23 sec	22 sec	21 sec	20 sec	19 sec	18 sec	17 sec	16 sec	15 sec	14 sec	13 sec	12 sec	11 sec	10 sec	9 sec	8 sec	7 sec	6 sec	5 sec	4 sec	3 sec	2 sec	1 sec
DT
54.9%	54.9%	54.2%	55.7%	55.7%	58.7%	57.6%	56.4%	54.2%	57.2%	61.0%	60.6%	56.1%	52.7%	56.1%	57.6%	54.5%	55.7%	55.7%	53.8%	58.0%	57.2%	62.5%	55.7%	59.5%	60.6%	60.6%	56.4%	54.5%	56.1%
bagging
61.4%	59.1%	60.2%	59.5%	59.1%	60.6%	61.4%	59.8%	59.5%	61.7%	59.5%	57.6%	58.0%	61.4%	59.5%	59.1%	57.6%	60.2%	61.0%	59.8%	61.4%	63.3%	61.0%	62.9%	64.8%	62.9%	64.0%	61.4%	62.9%	63.3%
adaboost
54.2%	54.2%	60.2%	58.0%	61.0%	59.8%	61.4%	56.1%	59.5%	63.6%	57.6%	58.0%	56.4%	55.7%	60.2%	58.0%	57.6%	56.8%	56.1%	58.7%	58.3%	56.1%	58.3%	57.6%	58.3%	61.4%	59.5%	59.5%	58.7%	61.0%
GBDT
60.6%	62.1%	60.6%	61.0%	58.7%	59.1%	62.1%	61.4%	61.0%	58.7%	61.4%	61.0%	61.0%	62.1%	59.8%	58.0%	61.0%	61.0%	61.7%	61.0%	62.9%	61.4%	63.3%	65.9%	66.7%	62.1%	65.9%	62.1%	64.0%	61.7%
XGB
61.0%	61.7%	62.1%	61.7%	60.2%	62.1%	62.5%	61.7%	60.6%	61.0%	60.2%	59.8%	61.0%	61.4%	60.6%	62.5%	62.1%	62.9%	62.5%	62.1%	63.6%	63.6%	61.7%	64.4%	65.2%	64.4%	64.4%	62.5%	64.0%	64.0%
RF
63.3%	61.7%	60.2%	64.0%	62.5%	60.6%	64.0%	58.7%	59.5%	61.4%	63.3%	61.0%	63.3%	61.0%	61.4%	61.4%	59.8%	59.8%	61.4%	62.1%	61.4%	62.5%	63.6%	62.9%	63.6%	64.4%	63.6%	65.2%	62.5%	65.2%
gcForest
62.9%	63.3%	61.7%	59.8%	61.0%	59.8%	61.4%	62.5%	63.6%	63.3%	63.6%	64.0%	61.4%	64.8%	62.1%	63.3%	61.4%	59.8%	62.5%	64.0%	63.6%	63.3%	62.1%	62.9%	64.4%	67.4%	65.5%	67.4%	65.2%	63.6%

ensemble results:
E1. the same ML method (horizontally) first and then ensemble vertically: 69.3%
E2. the same time interval (vertically) first and then horizontally: 70.5%

ensemble all 210 models: 69.7%

E3. RF: 63.8%
    gcForest	63.8%
E4. take the output of 210 trained models as input of DT: 65%
E5. take the first 2 layers nodes from DT: 68.6%
E6. take the first 3 layers nodes from DT: 67.0%

plots:
\begin{figure}
    \centering
    \includegraphics{Sections/oldresult.png}
    \caption{Caption}
    \label{fig:my_label}
\end{figure}
